# Supplementary material for: Microscopic Theory of Cation Exchange in CdSe Nanocrystals
Source: arXiv:1409.4832 ancillary file (2014-10-15)
Supplement: Supplementary file 1 [file SM_cdse-ag2se.pdf]

**Supplementary Information for:**  
**Microscopic Theory of Cation Exchange in CdSe Nanocrystals**

Florian D. Ott,<sup>1</sup> Leo L. Spiegel,<sup>1</sup> David J. Norris,<sup>1,\*</sup> and Steven C. Erwin<sup>2,†</sup>

<sup>1</sup>*Optical Materials Engineering Laboratory,  
ETH Zurich, 8092 Zurich, Switzerland*

<sup>2</sup>*Center for Computational Materials Science,  
Naval Research Laboratory, Washington, D.C. 20375, USA*

(Dated: November 15, 2014)

---

<sup>\*</sup>Electronic address: `dnorris@ethz.ch`

<sup>†</sup>Electronic address: `steve.erwin@nrl.navy.mil`

## I. BAND GAP OF BULK CADMIUM SELENIDE

To evaluate the binding energies of electrically active (donor and acceptor) impurity states, it is important to work within a theoretical framework which represents the band gap of the host (wurtzite CdSe) with good accuracy. The DFT band gap of CdSe in the PBE generalized-gradient approximation is 0.54 eV, which badly underestimates the experimental value of 1.84 eV [1]. To remedy this we used instead the screened hybrid functional of Heyd, Scuseria, and Ernzerhof (HSE) [2, 3]:

$$E_{\text{xc}}^{\text{HSE}} = aE_{\text{x}}^{\text{HF,SR}}(\omega) + (1 - a)E_{\text{x}}^{\text{PBE,SR}}(\omega) + E_{\text{x}}^{\text{PBE,LR}}(\omega) + E_{\text{c}}^{\text{PBE}}(\omega) \quad (\text{S.I.1})$$

with a range separation of  $\omega = 0.2 \text{ \AA}^{-1}$ . The commonly used value,  $a = 0.25$ , for the fraction of short-range Hartree-Fock exchange already results in a much more accurate band gap, 1.48 eV. For our work we set  $a = 0.34$ , which brings the band gap into essentially perfect agreement (1.85 eV) with experiment.

## II. DEFECT FORMATION ENERGIES AND CHARGE STATES

We evaluated the formation energies of interstitial Ag, substitutional Ag, and interstitial Cd ( $X$ ) in different charge states  $q$  in CdSe using the standard formalism [4–8]:

$$E_{\text{form}}(X^q) = E_{\text{tot}}(X^q) - \sum_i n_i \mu_i + q(E_F + \varepsilon^{\text{vbm}}) + q\Delta V - E_{\text{corr}}^q \quad (\text{S.II.1})$$

Here  $E_{\text{tot}}(X^q)$  is the total energy of the defect system,  $\mu_i$  is the chemical potential of atom type  $i$  ( $i = \text{Ag, Cd, Se}$ ) and  $n_i$  the corresponding number of atoms contained in the supercell. The chemical potentials of Cd and Se must obey the constraints

$$\mu_{\text{Cd}} + \mu_{\text{Se}} = \mu_{\text{CdSe}} \quad (\text{S.II.2})$$

$$\mu_{\text{Cd}} \leq \mu_{\text{Cd}}^0 \quad (\text{S.II.3})$$

$$\mu_{\text{Se}} \leq \mu_{\text{Se}}^0 \quad (\text{S.II.4})$$

where  $\mu_{\text{Cd}}^0$  and  $\mu_{\text{Se}}^0$  are the energies per atom in bulk Cd and Se, respectively. The chemical potentials of Ag, Cd, and Se do not affect the charge-transition levels and are therefore not

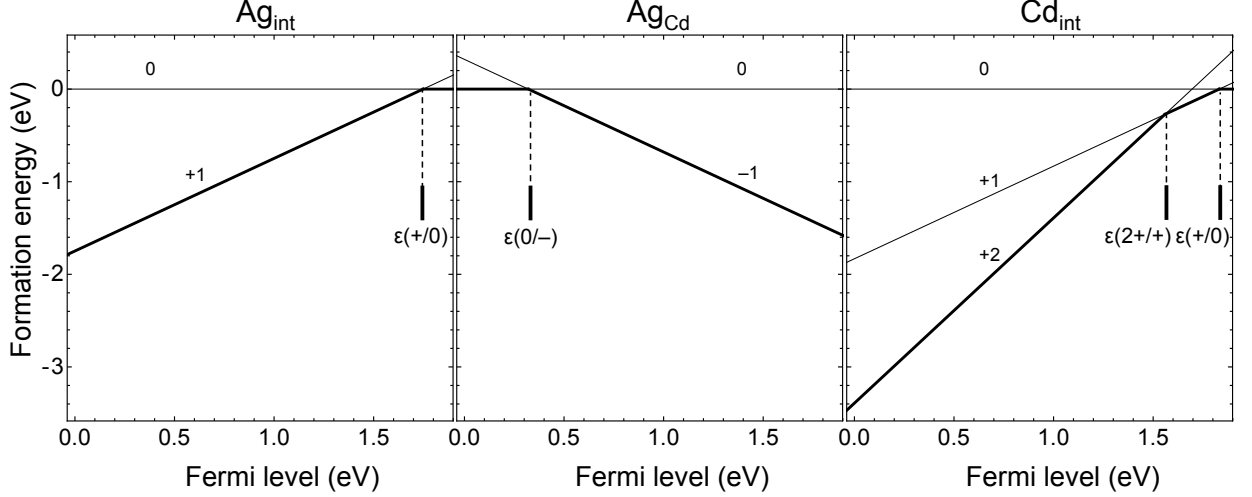

FIG. S.1: DFT/HSE formation energy of various Ag and Cd charge states (relative to the neutral charge state) versus Fermi level, referenced to the valence band maximum. The charge-transition levels  $\varepsilon(q_1/q_2)$  correspond to the Fermi level value where the formation energies for charge states  $q_1$  and  $q_2$  are equal.

of primary interest for our main focus, which is determine the stable charge states of Ag in CdSe.  $(E^{\text{Fermi}} + \varepsilon^{\text{vbm}})$  is the sum of the Fermi level (relative to the valence band maximum) and the valence band maximum.  $\Delta V$  is an alignment term which accounts for the shift of the reference electrostatic potential between the bulk and defect cells [8],

$$\Delta V = V^r(\text{bulk}) - V^r(X^0), \quad (\text{S.II.5})$$

where the reference potential in the defect supercell is defined far from the impurity. The correction energy  $E_{\text{corr}}^q$  accounts for the artificial interaction between the charged defect and its periodic images. We used the simplified expression for the first-order (monopole-monopole) plus third-order (monopole-quadrupole) image charge corrections of Lany and Zunger [6]:

$$E_{\text{corr}}^q = [1 + c_{\text{sh}} (1 - \varepsilon^{-1})] \frac{q^2 \alpha_{\text{M}}}{2\varepsilon \Omega^{1/3}} \quad (\text{S.II.6})$$

The shape factor  $c_{\text{sh}} = -0.37$  was obtained from evaluating the first and third order image charge correction terms of a point charge in a simple cubic cell [6], which is a good approximation for our orthorhombic cell ( $22.0 \text{ \AA} \times 22.8 \text{ \AA} \times 21.5 \text{ \AA}$ ). We used the theoretical dielectric constant,  $\varepsilon=7.87$ , computed here using density functional perturbation theory [9]. Finally,  $\alpha_{\text{M}}$  is the Madelung constant for a simple cubic system (2.8373), and  $\Omega$  is the volume

TABLE I: Defect type and donor/acceptor binding energies.

| Charge transition level         | Defect type | Binding energy (eV) |
|---------------------------------|-------------|---------------------|
| $\text{Ag}_{\text{int}} (+/0)$  | Donor       | 0.10                |
| $\text{Ag}_{\text{Cd}} (0/-)$   | Acceptor    | 0.32                |
| $\text{Cd}_{\text{int}} (2+/+)$ | Donor       | 0.29                |
| $\text{Cd}_{\text{int}} (+/0)$  | Donor       | 0.02                |

of the supercell.

Figure S.1 and Table I show our results for formation energies, charge-transition levels, and donor/acceptor binding energies of  $\text{Ag}_{\text{int}}$ ,  $\text{Ag}_{\text{Cd}}$ , and  $\text{Cd}_{\text{int}}$ . The primary results of interest for the study in the accompanying paper are qualitative and hence robust: when the Fermi levels falls within a wide window (from 0.3 to 1.5 eV above the valence band maximum) the stable charge states for  $\text{Ag}_{\text{int}}$ ,  $\text{Ag}_{\text{Cd}}$ , and  $\text{Ag}_{\text{int}}$  are +1, -1, and +2, respectively.

### III. ENERGETICS OF CLUSTERED SILVER IMPURITIES

In our study we used the kinetic Monte Carlo method to demonstrate that doping of Ag into CdSe nanocrystals eventually leads, by cation exchange, to the formation of  $\text{Ag}_2\text{Se}$ . We built into the KMC simulation several implicit assumptions about this process that call for more detailed justification. We discuss here the three most important of these assumptions, and show quantitative as well as qualitative evidence supporting them.

#### III.1. Atomistic structure of Ag clusters

Our first assumption is that a region of wurtzite CdSe, when fully doped with Ag, is indeed structurally and crystallographically similar to  $\text{Ag}_2\text{Se}$  in its naumannite phase. Figure S.2 shows three crystal structures that demonstrate the very close similarity between fully doped CdSe and naumannite  $\text{Ag}_2\text{Se}$ . The left structure (1) shows a region of idealized CdSe fully doped with one  $\text{Ag}_{\text{int}}$  and one  $\text{Ag}_{\text{Cd}}$  per Se atom, which creates the correct local stoichiometry  $\text{Ag}_2\text{Se}$ . The middle structure (2) shows this fully doped region at its equilibrium geometry, which is indeed only slightly distorted from the idealized structure. The right structure (3)

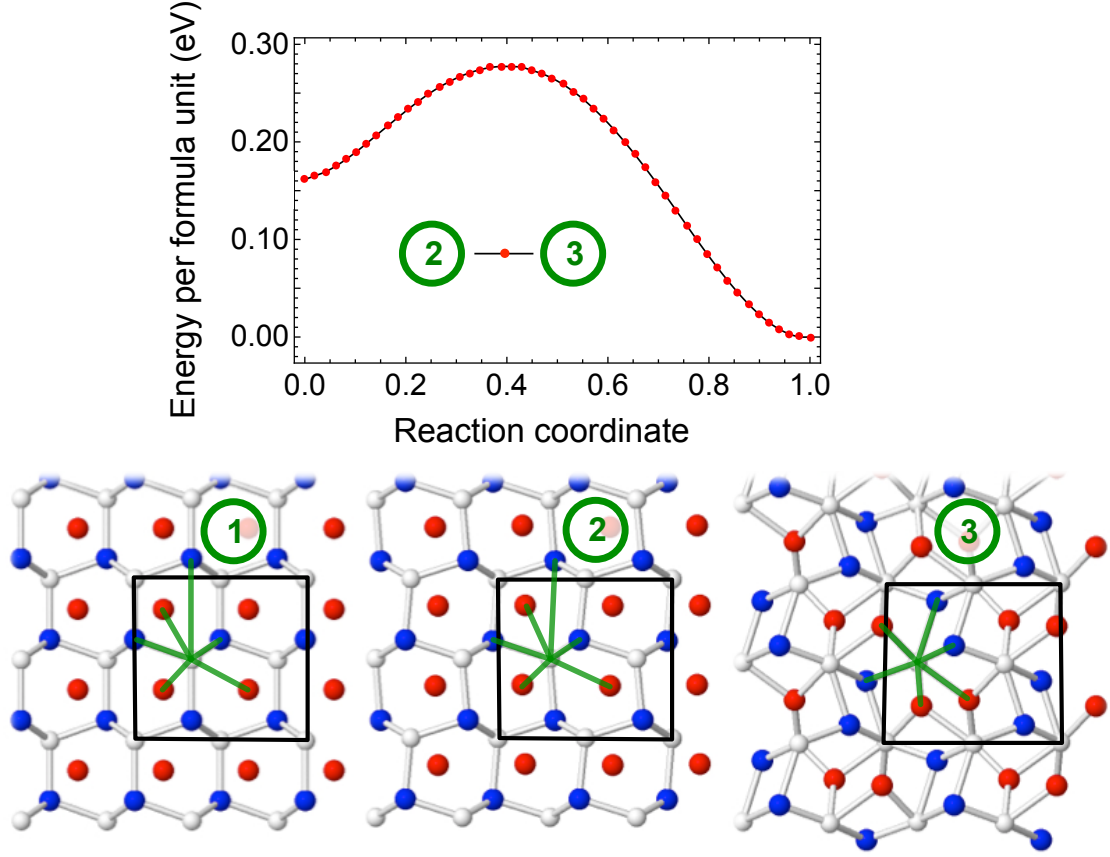

FIG. S.2: Energetics and structural models for the transformation of fully doped CdSe to naumannite  $\text{Ag}_2\text{Se}$ . See text for discussion.

shows  $\text{Ag}_2\text{Se}$  naumannite in its equilibrium structure.

To aid in visualizing the close relationship between structures (2) and (3) we use green line segments to highlight the local coordination around one Se atom. In structure (2) this consists of three  $\text{Ag}_{\text{int}}$  and three  $\text{Ag}_{\text{Cd}}$  atoms, while in structure (3) these impurities can be identified as the three crystallographic “ $\text{Ag}_{\text{I}}$ ” and three “ $\text{Ag}_{\text{II}}$ ” sites, respectively, of the naumannite crystal phase.

Finally, we show that structures (2) and (3) are also energetically close. Figure S.2 shows the total energy as structure (2) is transformed into structure (3) along the pathway of minimum energy, calculated within DFT/PBE using the nudged-elastic band method. There is a small activation barrier of 0.12 eV per  $\text{Ag}_2\text{Se}$  formula unit, and an overall energy gain (as expected) upon transformation to the naumannite phase.

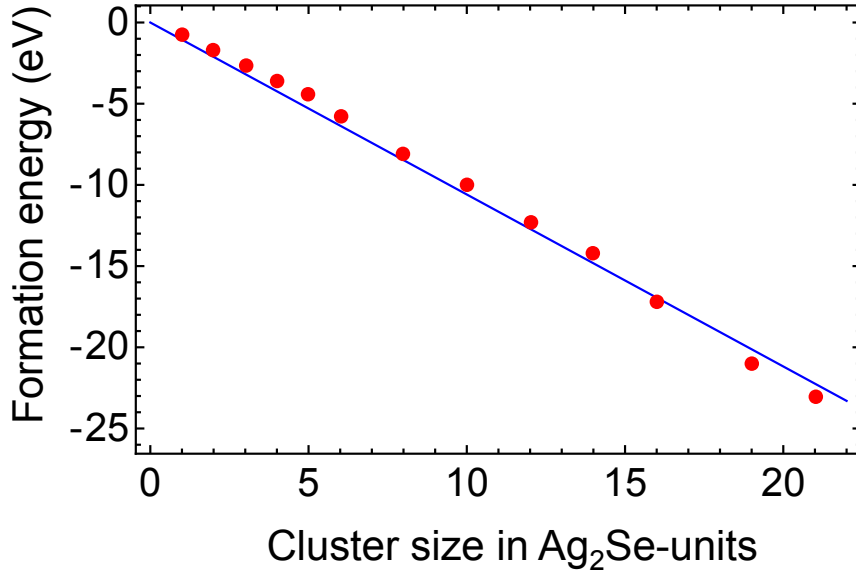

FIG. S.3: DFT/PBE formation energy per  $\text{Ag}_2\text{Se}$  formula unit of  $(\text{Ag}_2\text{Se})_n$  clusters as a function of cluster size  $n$ .

### III.2. Energetics of Ag clusters

Our second assumption is that the energy of a fully doped region of CdSe is represented with reasonable accuracy within our KMC model—that is, that the energy of a  $(\text{Ag}_2\text{Se})_n$  cluster is indeed given by  $n$  times the energy of one  $\text{Ag}_2\text{Se}$  unit.

To demonstrate the validity of this assumption we used DFT/PBE to compute the formation energies of  $(\text{Ag}_2\text{Se})_n$  clusters embedded in a wurtzite CdSe supercell of 360 atoms, for cluster sizes  $n = 1$  to 21. Figure S.3 shows that the energy of these clusters are indeed linearly proportional to  $n$ . This result, together with the structural results, establishes that our effective cluster expansion of the energy is a reasonable description of bulk  $\text{Ag}_2\text{Se}$ .

### III.3. Electrostatics of Ag clusters

The final assumption built into our simulations is that the stable charge state of a cluster  $(\text{Ag}_{\text{int}}^+)_n (\text{Ag}_{\text{Cd}}^-)_m \text{Se}_{2n}$  is given by the sum of the individual charges—that is, that the cluster has net charge  $n - m$ . In principle this issue could be investigated using the formalism of Sec. II, but in practice this is computationally prohibitive for large clusters. Instead we used a more direct approach by using DFT/PBE to compute the binding energy of a single impurity

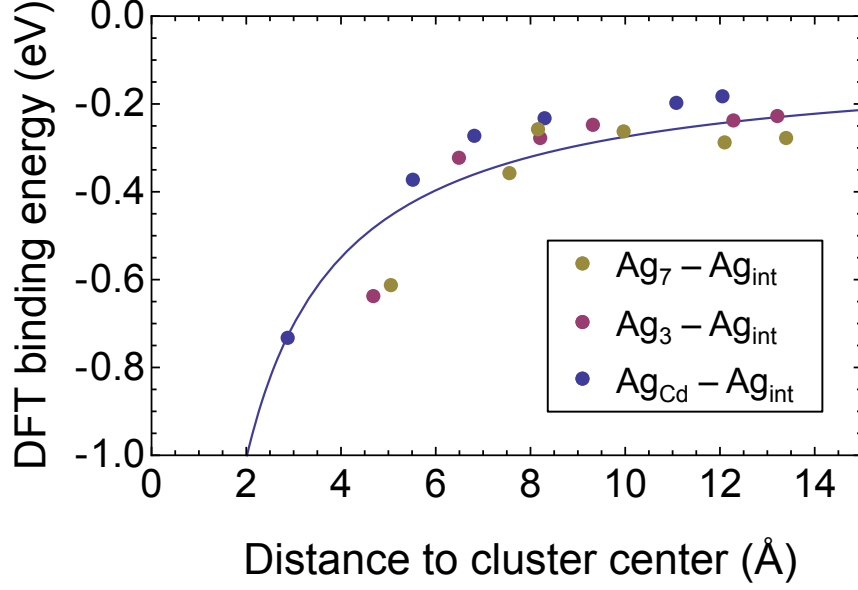

FIG. S.4: DFT/PBE binding energies of various charged Ag clusters with one  $\text{Ag}_{\text{int}}^+$  impurity, as a function of their separation.

in a known charge state to a cluster with unknown charge. For the single impurity we used  $\text{Ag}_{\text{int}}^+$ . We investigated two clusters,  $(\text{Ag}_{\text{int}})_1(\text{Ag}_{\text{Cd}})_2$  (denoted as  $\text{Ag}_3$ ) and  $(\text{Ag}_{\text{int}})_3(\text{Ag}_{\text{Cd}})_4$  (denoted as  $\text{Ag}_7$ ), and as a cross-check also used  $\text{Ag}_{\text{Cd}}^-$  to represent a one-atom cluster. All three clusters have the same putative charge state,  $n - m = -1$ .

Figure S.4 shows that the DFT/PBE binding energies are indeed attractive, as expected for oppositely charged objects. Moreover, the energies for all three clusters fall on the same curve, implying that they carry the same  $-1$  charge. This result validates our assumption the charge state of a cluster is the sum of the individual charges.

#### IV. INTERACTIONS FROM DIELECTRIC POLARIZATION OF THE SURFACE

For a set of  $N$  point charges  $\{q_1, q_2, \dots, q_N\}$  in a dielectric sphere ( $\varepsilon_1$ ) with radius  $R$  which is embedded in another dielectric material ( $\varepsilon_2$ ), the electrostatic energy is given by [10]:

$$E_{\text{Coul}} = \sum_{i=1}^N \sum_{j>i}^N \frac{q_i q_j}{\varepsilon_1 r_{ij}} + \underbrace{\frac{\varepsilon_1 - \varepsilon_2}{\varepsilon_1} \sum_{i=1}^N \sum_{j=1}^N q_i q_j \sum_{l=0}^{\infty} \frac{l+1}{\varepsilon_1 l + \varepsilon_2 (l+1)} \frac{r_i^l r_j^l}{R^{2l+1}} P_l(\cos \theta_{ij})}_{E_{\text{Pol}}} \quad (\text{S.IV.1})$$

where  $r_i$  is the distance from  $q_i$  to the center of the sphere,  $r_{ij}$  is the distance from  $q_i$  to  $q_j$  and  $\theta_{ij}$  is the angle between  $q_i$  and  $q_j$  with respect to the center of the sphere. The polarization energy  $E_{\text{Pol}}$  can be reproduced by placing image charges outside the sphere for each point charge in the sphere [11]. By applying the method of image charges,  $E_{\text{Pol}}$  can be expressed as:

$$E_{\text{Pol}} = \sum_{i=1}^N \frac{q_i}{\varepsilon_1} \sum_{j=1}^N \int_R^{\infty} \frac{\rho_j(z)}{\sqrt{z^2 + r_i^2 - 2zr_i \cos \theta_{ij}}} dz \quad (\text{S.IV.2})$$

with the image charge  $\rho_j(z)$ . Using the generating function for Legendre polynomials

$$\frac{1}{\sqrt{1 - 2xu + u^2}} = \sum_{l=0}^{\infty} u^l P_l(x) \quad (\text{S.IV.3})$$

we can rewrite equation S.IV.2:

$$E_{\text{Pol}} = \sum_{i=1}^N \frac{q_i}{\varepsilon_1} \sum_{j=1}^N \sum_{l=0}^{\infty} r_i^l P_l(\cos \theta_{ij}) \int_R^{\infty} \frac{\rho_j(z)}{z^{l+1}} dz \quad (\text{S.IV.4})$$

The image charge distribution can be found by setting the second term of Eq. S.IV.1 ( $E_{\text{Pol}}$ ) and Eq. S.IV.4 equal. The resulting image charge consists of a point charge ( $q_P$ ) and a distributed charge ( $q_D$ ) both of the same sign as  $q_j$  [11]:

$$\rho_j(z) = q_j \frac{\varepsilon_1 - \varepsilon_2}{\varepsilon_1 + \varepsilon_2} \left[ \underbrace{\frac{R}{r_j} \delta\left(z - \frac{R^2}{r_j}\right)}_{q_P} + \underbrace{\frac{\varepsilon_1 q_j}{R} \left(\frac{r_j z}{R^2}\right)^{-\frac{\varepsilon_2}{\varepsilon_1 + \varepsilon_2}} H\left(z - \frac{R^2}{r_j}\right)}_{q_D} \right] \quad (\text{S.IV.5})$$

with  $\delta(x)$  being the Dirac delta function and  $H(x)$  the Heaviside step function. In this form we clearly can see that the interaction between a point charge and its image is always repulsive, and this interaction increases as the charge approaches the surface of the nanocrystal.

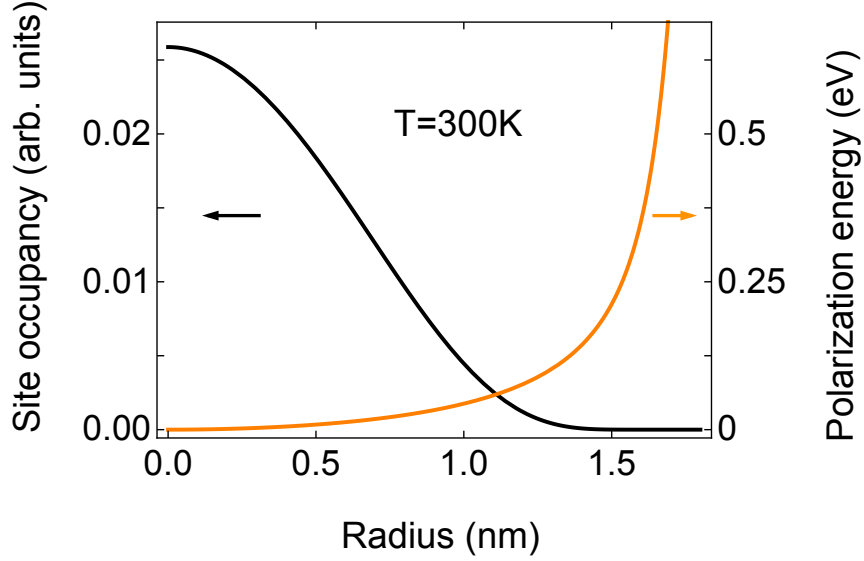

FIG. S.5: Polarization energy (orange line) and the corresponding concentration distribution (black line) at 300 K for a single elementary charge in a dielectric sphere ( $\epsilon_1 = 9$ ) with a diameter of 3.5 nm.

Figure S.5 shows the electrostatic energy due to the polarization effect (orange curve) of a elementary point charge in a dielectric sphere ( $\epsilon_1 = 9$ ) with a diameter of 3.5 nm which is embedded in another dielectric material. For the dielectric constant of the surrounding material we used a value of  $\epsilon_2 = 2$  which corresponds to a typical non-polar solvent (*e.g.* hexane).

## V. THE EFFECT OF COUNTERIONS IN THE SOLVENT

In our simulations, the number  $N$  of entering  $\text{Ag}^+$  ions may not always be precisely balanced by  $N/2$  departing  $\text{Cd}^{2+}$  ions—although this ratio is indeed enforced on average as the nanocrystal converts to  $\text{Ag}_2\text{Se}$ . In such transient situations the nanocrystal has a net charge which must be compensated by external counterions. We regarded these counterions as very mobile because they are in solution. For this reason we considered them as being uniformly smeared out in the vicinity of the nanocrystal. Such a uniform charge distribution does not affect the potential-energy landscape for reactions inside the nanocrystal.

One could hypothesize that the opposite limit might be more appropriate: that counterions are strongly attracted to their image charges (or to the real charges) inside the nanocrystal, and thus strongly alter the potential-energy landscape for reactions inside. To

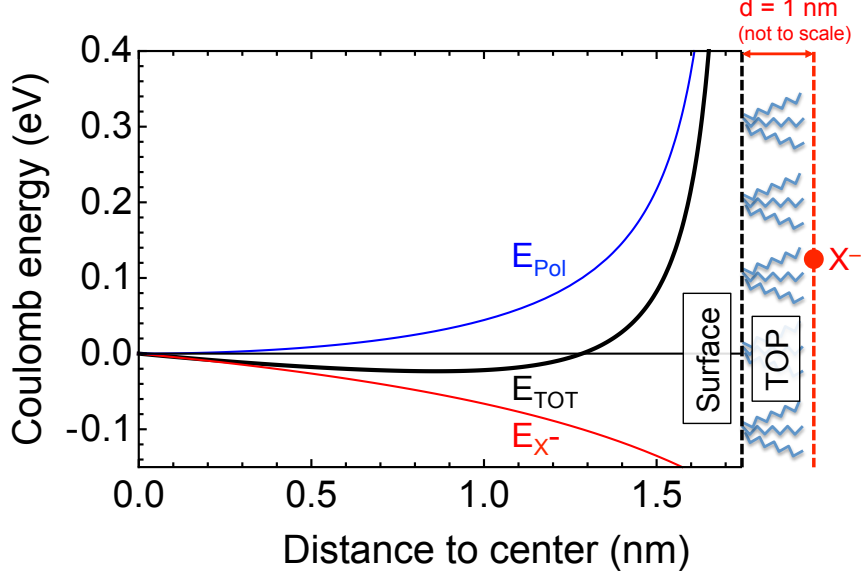

FIG. S.6: Electrostatic interaction of an interior point charge with an exterior point counterion  $X^-$ .  $E_{\text{Pol}}$  is the interaction of the interior charge with its own image charge (which represents the effect of surface polarization),  $E_{X^-}$  is the interaction energy of the interior charge with the exterior counterion, and  $E_{\text{TOT}}$  is their sum. The distance (1 nm) of the counterion from the surface of the nanocrystal takes into consideration the size of a typical ligand such as trioctylphosphine (TOP).

address this question, we performed a simple electrostatic calculation to estimate how the potential energy of a single ion inside the nanocrystal would be affected by the presence of a counterion just outside the nanocrystal. The result, shown in Fig. S.6, is that this effect, while not zero, is reasonably small—and does not qualitatively change our finding that interior ions are strongly repelled from the surface of the nanocrystal.

## VI. SUPPLEMENTARY MOVIE

Figure S.7 is a snapshot from a typical kinetic Monte Carlo simulation run. The complete video is also available as part of the supplementary information.

The nanocrystal has a diameter of 3.5 nm. On the left-hand side one can observe the dynamics of the Ag impurities and on the right-hand side data about the running simulation. The bar plot presents the statistical concentration distribution of impurities binned into 5 different atomic shells, evaluated from 100 separate simulation runs.

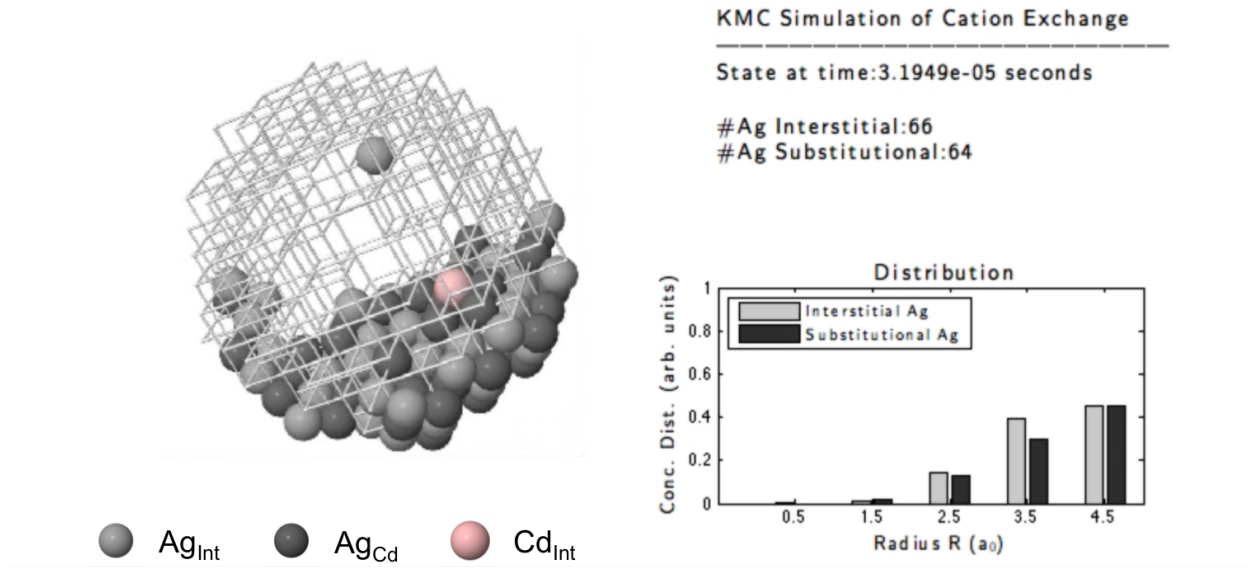

FIG. S.7: Snapshot from a kinetic Monte Carlo simulation.

- 
- [1] L. Ley, R. A. Pollak, F. R. McFeely, S. P. Kowalczyk, and D. A. Shirley, Phys. Rev. B **9**, 600 (1974).
  - [2] J. Heyd, G. E. Scuseria, and M. Ernzerhof, J. Chem. Phys. **118**, 8207 (2003).
  - [3] J. Heyd, G. E. Scuseria, and M. Ernzerhof, J. Chem. Phys. **124**, 219906 (2006).
  - [4] C. G. Van de Walle, D. B. Laks, G. F. Neumark, and S. T. Pantelides, Phys. Rev. B **47**, 9425 (1993).
  - [5] C. G. Van de Walle, and J. Neugebauer, J. Appl. Phys. **95**, 3851 (2004).
  - [6] S. Lany, and A. Zunger, Modelling Simul. Mater. Sci. Eng. **17**, 084002 (2009).
  - [7] C. Freysoldt, J. Neugebauer, and C. G. Van de Walle, Phys. Status Solidi B **248**, 1067 (2011).
  - [8] H.-P. Komsa, T. T. Rantala, and A. Pasquarello, Phys. Rev. B **86**, 045112 (2012).
  - [9] X. Wu, D. Vanderbilt, and D. R. Hamann, Phys. Rev. B **72**, 035105 (2005).
  - [10] V. V. Batygin and I. N. Toptygin, *Problems in Electrodynamics* (Academic Press, 1964).
  - [11] W. T. Norris, IEE Proc. - Sci. Meas. Technol. **142**, 142 (1995).
